# Supplementary material for: Exploring the Impact of Model Scaling on Parameter-Efficient Tuning
Source: arXiv:2306.02320 source file (2023-12-10)
Supplement: Supplementary file 1 [file appendix_table.tex]

\begin{table*}[!th]
{\small
\begin{adjustbox}{max width=1\linewidth}
{
\setlength\tabcolsep{0.3em}
\begin{tabular}{l|l|*{3}{d{3.2}}|*{3}{d{3.2}}|*{2}{d{3.2}}|*{1}{d{3.2}}|*{2}{d{3.2}}|*{2}{d{3.2}}||*{3}{d{3.2}}|*{3}{d{3.2}}|*{2}{d{3.2}}}
\toprule
  \multicolumn{1}{l|}{\textbf{Task Category}} &
  \multicolumn{1}{c|}{- -} &
  \multicolumn{3}{c|}{\textbf{SA} (3 tasks)} & \multicolumn{3}{c|}{\textbf{NLI} (3 tasks)} & \multicolumn{2}{c|}{\textbf{PI} (2 tasks)} & \multicolumn{1}{c|}{\textbf{QA} (1 task)} & \multicolumn{2}{c|}{\textbf{SUM} (2 tasks)} &
  \multicolumn{2}{c|}{- -} &
  \multicolumn{3}{c|}{\textbf{SA} (3 tasks)} & \multicolumn{3}{c|}{\textbf{NLI} (3 tasks)} & \multicolumn{2}{c}{\textbf{PI} (2 tasks)} 
  \\
  \midrule
   \multicolumn{1}{l|}{\textbf{Task}} &
  \multicolumn{1}{c|}{- -} & \multicolumn{1}{c}{SST2} &
  \multicolumn{1}{c}{IMDB} & \multicolumn{1}{c|}{\makecell{Rotten\\Tomatoes}} & \multicolumn{1}{c}{MNLI} & \multicolumn{1}{c}{QNLI} & \multicolumn{1}{c|}{RTE} & \multicolumn{1}{c}{MRPC} & \multicolumn{1}{c|}{QQP} & \multicolumn{1}{c|}{NQ-Open} & \multicolumn{1}{c}{SAMSum} & \multicolumn{1}{c|}{Multi-News} & \multicolumn{2}{c|}{- -}  & \multicolumn{1}{c}{SST2}  & \multicolumn{1}{c}{IMDB}  & \multicolumn{1}{c|}{\makecell{Rotten\\Tomatoes}}  & \multicolumn{1}{c}{MNLI}  & \multicolumn{1}{c}{QNLI}  & \multicolumn{1}{c|}{RTE}  & \multicolumn{1}{c}{MRPC}  & \multicolumn{1}{c}{QQP} \\
  \midrule
  \multicolumn{1}{l|}{\textbf{Metric}} &
  \multicolumn{1}{c|}{- -} &
  \multicolumn{3}{c|}{Acc.} & \multicolumn{3}{c|}{Acc.} & \multicolumn{2}{c|}{Acc.} & \multicolumn{1}{c|}{F1.} & \multicolumn{2}{c|}{ROUGE-L} & \multicolumn{2}{c|}{- -} & \multicolumn{3}{c|}{Acc.} & \multicolumn{3}{c|}{Acc.} & \multicolumn{2}{c}{Acc.} \\
\midrule
  \multicolumn{1}{l|}{\textbf{Backbone}} & \multicolumn{1}{c|}{- -} & \multicolumn{11}{c|}{\textbf{T5\quad\quad\quad}} &
  \multicolumn{2}{c|}{- -} & \multicolumn{8}{c}{\textbf{BERT\quad\quad\quad}} \\
\midrule
\midrule
\multicolumn{1}{l|}{\textbf{Scale}} &
\multicolumn{1}{c|}{- -} &
\multicolumn{11}{c|}{\TSMALL} &
  \multicolumn{2}{c|}{- -} & \multicolumn{8}{c}{\BERTSMALL} \\
\midrule
\multicolumn{1}{l|}{\textbf{Methods}} &
\multicolumn{1}{c|}{\textbf{Ratio}} & \multicolumn{11}{c|}{} & \multicolumn{2}{c|}{\textbf{Ratio}} & \multicolumn{8}{c}{} \\
\midrule

\multicolumn{1}{l|}{\textbf{Fine-tune}} & \multicolumn{1}{c|}{\textbf{1}} & \mc{91.8} & \mc{89.2} & \mcl{82.6} & \mc{82.4} & \mc{90.3} & \mcl{69.9} & \mc{89.7} & \mcl{88.0} & \mcl{7.0} & \mc{42.8} & \mcl{25.1} & \mctwol{\textbf{1}} & \mc{88.1} & \mc{86.0} & \mcl{81.6} & \mc{72.9} & \mc{87.1} & \mcl{63.8} & \mc{80.6} & \mc{85.8} \\ 
\midrule
% \multicolumn{1}{l|}{\textbf{Prompt}} & \multicolumn{1}{c|}{\multirow{3}{*}{\textbf{0.01}}} & \mctwo{} & \mctwo{} & \mctwo{} & \mctwo{} & \mctwol{} & \mctwo{} & \mctwol{} & \mctwol{} & \mctwo{} & \mctwo{} & \mctwol{} & \mctwo{} & \mctwo{} \\ 
\multicolumn{1}{l|}{\textbf{\AFPADJACENTExternal}} & \multicolumn{1}{c|}{\multirow{2}{*}{0.07\%}} & \mc{74.0} & \mc{85.8} & \mcl{59.1} & \mc{77.2} & \mc{80.8} & \mcl{58.1} & \mc{77.2} & \mcl{80.0} & \mcl{2.1} & \mc{27.1} & \mcl{20.3} & \mctwol{\multirow{2}{*}{0.09\%}} & \mc{78.2} & \mc{73.7} & \mcl{74.3} & \mc{64.2} & \mc{79.3} & \mcl{59.1} & \mc{76.8} & \mc{75.1} \\
\multicolumn{1}{l|}{\textbf{\AFPADJACENTInternal}} & \multicolumn{1}{c|}{} & \mc{76.3} & \mc{81.5} & \mcl{78.0} & \mc{72.5} & \mc{80.4} & \mcl{57.9} & \mc{80.9} & \mcl{79.8} & \mcl{3.5} & \mc{33.4} & \mcl{22.9} & \mctwol{} & \mc{77.2} & \mc{74.3} & \mcl{74.8} & \mc{63.3} & \mc{79.9} & \mcl{65.6} & \mc{79.0} & \mc{77.4} \\
\midrule
% \multicolumn{1}{l|}{\textbf{Bitfit}} & \multicolumn{1}{c|}{\multirow{3}{*}{\textbf{0.01}}} & \mctwo{} & \mctwo{} & \mctwo{} & \mctwo{} & \mctwol{} & \mctwo{} & \mctwol{} & \mctwol{} & \mctwo{} & \mctwo{} & \mctwol{} & \mctwo{} & \mctwo{}\\ 
\multicolumn{1}{l|}{\textbf{\AFPADJACENTExternal}} & \multicolumn{1}{c|}{\multirow{2}{*}{0.16\%}} & \mc{86.4} & \mc{81.4} & \mcl{78.0} & \mc{72.9} & \mc{83.6} & \mcl{61.4} & \mc{75.5} & \mcl{84.9} & \mcl{2.0} & \mc{35.8} & \mcl{24.1} & \mctwol{\multirow{2}{*}{0.05\%}} & \mc{81.4} & \mc{86.3} & \mcl{80.1} & \mc{81.3} & \mc{81.2} & \mcl{60.3} & \mc{85.7} & \mc{60.9} \\
\multicolumn{1}{l|}{\textbf{\AFPADJACENTInternal}} & \multicolumn{1}{c|}{} & \mc{76.3} & \mc{81.5} & \mcl{78.0} & \mc{72.5} & \mc{80.4} & \mcl{57.9} & \mc{80.9} & \mcl{79.8} & \mcl{3.5} & \mc{33.9} & \mcl{22.9} & \mctwol{} & \mc{80.1} & \mc{85.2} & \mcl{78.0} & \mc{68.1} & \mc{84.6} & \mcl{59.4} & \mc{80.9} & \mc{79.0} \\
\midrule

% \multicolumn{1}{l|}{\textbf{Lora}} & 
\multicolumn{1}{l|}{\textbf{\AFPADJACENTExternal}} & \multicolumn{1}{c|}{\multirow{2}{*}{0.30\%}} & \mc{89.3} & \mc{89.9} & \mcl{85.3} & \mc{71.1} & \mc{85.6} & \mcl{64.9} & \mc{82.1} & \mcl{79.2} & \mcl{3.8} & \mc{38.0} & \mcl{22.7} & \mctwol{{\multirow{2}{*}{0.23\%}}} & \mc{88.1} & \mc{85.6} & \mcl{81.6} & \mc{72.8} & \mc{86.2} & \mcl{66.8} & \mc{81.4} & \mc{85.3} \\
\multicolumn{1}{l|}{\textbf{\AFPADJACENTInternal}} & \multicolumn{1}{c|}{} & \mc{82.0} & \mc{84.9} & \mcl{80.1} & \mc{59.8} & \mc{78.3} & \mcl{59.9} & \mc{79.7} & \mcl{75.3} & \mcl{3.0} & \mc{29.8} & \mcl{20.7} & \mctwol{} & \mc{84.1} & \mc{83.1} & \mcl{79.9} & \mc{65.7} & \mc{83.2} & \mcl{64.3} & \mc{80.6} & \mc{79.5} \\
\midrule

% \multicolumn{1}{l|}{\textbf{Adapter}} & \multicolumn{1}{c|}{\multirow{3}{*}{\textbf{0.01}}} & \mctwo{} & \mctwo{} & \mctwo{} & \mctwo{} & \mctwol{} & \mctwo{} & \mctwol{} & \mctwol{} & \mctwo{} & \mctwo{} & \mctwol{} & \mctwo{} & \mctwo{}\\ 
\multicolumn{1}{l|}{\textbf{\AFPADJACENTExternal}} & \multicolumn{1}{c|}{\multirow{2}{*}{1.04\%}} & \mc{92.2} & \mc{87.0} & \mcl{87.2} & \mc{83.8} & \mc{89.7} & \mcl{66.1} & \mc{84.8} & \mcl{89.3} & \mcl{7.9} & \mc{43.5} & \mcl{25.2} & \mctwol{{\multirow{2}{*}{0.70\%}}} & \mc{86.4} & \mc{93.1} & \mcl{84.5} & \mc{84.8} & \mc{87.8} & \mcl{64.3} & \mc{87.1} & \mc{66.8} \\
\multicolumn{1}{l|}{\textbf{\AFPADJACENTInternal}} & \multicolumn{1}{c|}{} & \mc{83.6} & \mc{81.8} & \mcl{74.3} & \mc{77.0} & \mc{83.8} & \mcl{59.1} & \mc{81.8} & \mcl{83.9} & \mcl{3.2} & \mc{38.6} & \mcl{23.7} & \mctwol{} & \mc{85.1} & \mc{92.5} & \mcl{81.6} & \mc{74.9} & \mc{85.7} & \mcl{65.4} & \mc{83.1} & \mc{85.2} \\
\midrule

% \multicolumn{1}{l|}{\textbf{Prefix}} & \multicolumn{1}{c|}{\multirow{3}{*}{\textbf{0.01}}} & \mctwo{} & \mctwo{} & \mctwo{} & \mctwo{} & \mctwol{} & \mctwo{} & \mctwol{} & \mctwol{} & \mctwo{} & \mctwo{} & \mctwol{} & \mctwo{} & \mctwo{}\\ 
% \multicolumn{1}{l|}{\textbf{\AFPADJACENTExternal}} & \multicolumn{1}{c|}{\multirow{2}{*}{1.82e-01}} & \mc{89.8} & \mc{86.1} & \mcl{85.9} & \mc{83.8} & \mc{89.3} & \mcl{69.0} & \mc{87.0} & \mcl{89.7} & \mcl{8.1} & \mc{43.6} & \mcl{25.1} & \mctwol{\multirow{2}{*}{1.84e-01}} & \mc{86.1} & \mc{85.9} & \mcl{81.0} & \mc{72.3} & \mc{86.4} & \mcl{63.7} & \mc{82.3} & \mc{83.4} \\
% \multicolumn{1}{l|}{\textbf{\AFPADJACENTInternal}} & \multicolumn{1}{c|}{} & \mc{89.9} & \mc{89.3} & \mcl{86.7} & \mc{83.3} & \mc{88.9} & \mcl{64.9} & \mc{88.0} & \mcl{87.3} & \mcl{6.8} & \mc{34.7} & \mcl{24.9} & \mctwol{} & \mc{87.7} & \mc{85.5} & \mcl{81.4} & \mc{71.1} & \mc{87.0} & \mcl{62.7} & \mc{80.0} & \mc{83.3} \\
% \midrule

\midrule
\multicolumn{1}{l|}{\textbf{Scale}} &
\multicolumn{1}{c|}{- -} &
\multicolumn{11}{c|}{\TBASE} &
  \multicolumn{2}{c|}{- -} & \multicolumn{8}{c}{\BERTBASE} \\
\midrule
\multicolumn{1}{l|}{\textbf{Methods}} &
\multicolumn{1}{c|}{\textbf{Ratio}} & \multicolumn{11}{c|}{} & \multicolumn{2}{c|}{\textbf{Ratio}} & \multicolumn{8}{c}{} \\
\midrule

\multicolumn{1}{l|}{\textbf{Fine-tune}} & \multicolumn{1}{c|}{\textbf{1}} & \mc{95.2} & \mc{90.3} & \mcl{86.6} & \mc{87.1} & \mc{93.7} & \mcl{80.1} & \mc{88.0} & \mcl{89.4} & \mcl{13.1} & \mc{45.6} & \mcl{26.1} & \mctwol{\textbf{1}} & \mc{92.3} & \mc{89.0} & \mcl{86.7} & \mc{81.7} & \mc{91.1} & \mcl{67.5} & \mc{86.5} & \mc{88.3} \\ 
\midrule
% \multicolumn{1}{l|}{\textbf{Prompt}} & \multicolumn{1}{c|}{\multirow{3}{*}{\textbf{0.01}}} & \mctwo{} & \mctwo{} & \mctwo{} & \mctwo{} & \mctwol{} & \mctwo{} & \mctwol{} & \mctwol{} & \mctwo{} & \mctwo{} & \mctwol{} & \mctwo{} & \mctwo{} \\ 
\multicolumn{1}{l|}{\textbf{\AFPADJACENTExternal}} & \multicolumn{1}{c|}{\multirow{2}{*}{0.03\%}} & \mc{83.5} & \mc{83.4} & \mcl{81.8} & \mc{83.8} & \mc{78.5} & \mcl{63.5} & \mc{82.2} & \mcl{82.5} & \mcl{1.5} & \mc{42.8} & \mcl{20.6} & \mctwol{\multirow{2}{*}{0.07\%}} & \mc{81.3} & \mc{83.9} & \mcl{78.4} & \mc{77.1} & \mc{78.4} & \mcl{68.3} & \mc{81.2} & \mc{60.3} \\
\multicolumn{1}{l|}{\textbf{\AFPADJACENTInternal}} & \multicolumn{1}{c|}{} & \mc{78.1} & \mc{80.8} & \mcl{72.0} & \mc{83.9} & \mc{59.5} & \mcl{63.8} & \mc{77.1} & \mcl{65.7} & \mcl{5.3} & \mc{42.7} & \mcl{25.0} & \mctwol{} & \mc{82.0} & \mc{84.2} & \mcl{79.3} & \mc{76.5} & \mc{78.0} & \mcl{69.2} & \mc{82.0} & \mc{59.4} \\
\midrule
% \multicolumn{1}{l|}{\textbf{Bitfit}} & \multicolumn{1}{c|}{\multirow{3}{*}{\textbf{0.01}}} & \mctwo{} & \mctwo{} & \mctwo{} & \mctwo{} & \mctwol{} & \mctwo{} & \mctwol{} & \mctwol{} & \mctwo{} & \mctwo{} & \mctwol{} & \mctwo{} & \mctwo{}\\ 
\multicolumn{1}{l|}{\textbf{\AFPADJACENTExternal}} & \multicolumn{1}{c|}{\multirow{2}{*}{0.11\%}} & \mc{93.6} & \mc{88.4} & \mcl{88.9} & \mc{86.1} & \mc{90.7} & \mcl{70.8} & \mc{85.1} & \mcl{88.8} & \mcl{6.7} & \mc{45.3} & \mcl{25.6} & \mctwol{\multirow{2}{*}{0.06\%}} & \mc{83.6} & \mc{84.2} & \mcl{80.6} & \mc{80.0} & \mc{81.2} & \mcl{68.7} & \mc{83.7} & \mc{61.1} \\
\multicolumn{1}{l|}{\textbf{\AFPADJACENTInternal}} & \multicolumn{1}{c|}{} & \mc{78.1} & \mc{80.8} & \mcl{72.0} & \mc{83.9} & \mc{59.5} & \mcl{58.8} & \mc{77.1} & \mcl{65.7} & \mcl{5.3} & \mc{42.7} & \mcl{24.9} & \mctwol{} & \mc{82.2} & \mc{83.3} & \mcl{79.4} & \mc{78.4} & \mc{80.0} & \mcl{68.5} & \mc{82.6} & \mc{58.3} \\
\midrule

% \multicolumn{1}{l|}{\textbf{Lora}}
\multicolumn{1}{l|}{\textbf{\AFPADJACENTExternal}} & \multicolumn{1}{c|}{\multirow{2}{*}{0.24\%}} & \mc{84.9} & \mc{61.8} & \mcl{82.1} & \mc{72.5} & \mc{87.2} & \mcl{53.1} & \mc{75.3} & \mcl{80.4} & \mcl{6.5} & \mc{44.5} & \mcl{25.4} & \mctwol{\multirow{2}{*}{0.27\%}} & \mc{92.1} & \mc{88.3} & \mcl{86.5} & \mc{80.8} & \mc{90.7} & \mcl{68.2} & \mc{86.3} & \mc{87.7} \\
\multicolumn{1}{l|}{\textbf{\AFPADJACENTInternal}} & \multicolumn{1}{c|}{} & \mc{93.0} & \mc{83.4} & \mcl{80.8} & \mc{78.4} & \mc{88.9} & \mcl{64.6} & \mc{78.0} & \mcl{87.5} & \mcl{5.9} & \mc{42.1} & \mcl{25.1} & \mctwol{} & \mc{90.9} & \mc{87.9} & \mcl{85.8} & \mc{76.5} & \mc{88.5} & \mcl{72.6} & \mc{87.7} & \mc{84.6} \\
\midrule

% \multicolumn{1}{l|}{\textbf{Adapter}} & \multicolumn{1}{c|}{\multirow{3}{*}{\textbf{0.01}}} & \mctwo{} & \mctwo{} & \mctwo{} & \mctwo{} & \mctwol{} & \mctwo{} & \mctwol{} & \mctwol{} & \mctwo{} & \mctwo{} & \mctwol{} & \mctwo{} & \mctwo{}\\ 
\multicolumn{1}{l|}{\textbf{\AFPADJACENTExternal}} & \multicolumn{1}{c|}{\multirow{2}{*}{0.73\%}} & \mc{94.9} & \mc{85.4} & \mcl{82.3} & \mc{87.9} & \mc{84.6} & \mcl{67.0} & \mc{82.8} & \mcl{85.4} & \mcl{10.0} & \mc{44.0} & \mcl{26.1} & \mctwol{\multirow{2}{*}{0.83\%}} & \mc{88.0} & \mc{91.1} & \mcl{86.0} & \mc{84.7} & \mc{87.0} & \mcl{70.0} & \mc{87.8} & \mc{66.7} \\
\multicolumn{1}{l|}{\textbf{\AFPADJACENTInternal}} & \multicolumn{1}{c|}{} & \mc{93.0} & \mc{83.4} & \mcl{80.8} & \mc{78.4} & \mc{88.9} & \mcl{64.6} & \mc{78.0} & \mcl{87.5} & \mcl{5.9} & \mc{42.1} & \mcl{25.1} & \mctwol{} & \mc{86.4} & \mc{89.0} & \mcl{83.1} & \mc{83.9} & \mc{85.4} & \mcl{69.9} & \mc{86.4} & \mc{63.0} \\
\midrule

% \multicolumn{1}{l|}{\textbf{Prefix}} & \multicolumn{1}{c|}{\multirow{3}{*}{\textbf{0.01}}} & \mctwo{} & \mctwo{} & \mctwo{} & \mctwo{} & \mctwol{} & \mctwo{} & \mctwol{} & \mctwol{} & \mctwo{} & \mctwo{} & \mctwol{} & \mctwo{} & \mctwo{}\\ 
% \multicolumn{1}{l|}{\textbf{\AFPADJACENTExternal}} & \multicolumn{1}{c|}{\multirow{2}{*}{9.67e-02}} & \mc{94.3} & \mc{86.3} & \mcl{88.0} & \mc{87.8} & \mc{92.5} & \mcl{70.1} & \mc{84.6} & \mcl{88.0} & \mcl{12.8} & \mc{44.2} & \mcl{26.0} & \mctwol{\multirow{2}{*}{1.14e-01}} & \mc{88.2} & \mc{92.2} & \mcl{84.8} & \mc{84.4} & \mc{87.7} & \mcl{71.3} & \mc{86.9} & \mc{68.7} \\
% \multicolumn{1}{l|}{\textbf{\AFPADJACENTInternal}} & \multicolumn{1}{c|}{} & \mc{94.4} & \mc{86.3} & \mcl{87.0} & \mc{86.3} & \mc{91.5} & \mcl{68.9} & \mc{81.3} & \mcl{90.0} & \mcl{9.5} & \mc{44.4} & \mcl{25.8} & \mctwol{} & \mc{88.7} & \mc{91.9} & \mcl{85.1} & \mc{84.9} & \mc{86.6} & \mcl{70.4} & \mc{87.4} & \mc{66.5} \\
% \midrule

\midrule
\multicolumn{1}{l|}{\textbf{Scale}} &
\multicolumn{1}{c|}{- -} &
\multicolumn{11}{c|}{\TXXL} &
  \multicolumn{2}{c|}{- -} & \multicolumn{8}{c}{\BERTLARGE} \\
\midrule
\multicolumn{1}{l|}{\textbf{Methods}} &
\multicolumn{1}{c|}{\textbf{Ratio}} & \multicolumn{11}{c|}{} & \multicolumn{2}{c|}{\textbf{Ratio}} & \multicolumn{8}{c}{} \\
\midrule
\multicolumn{1}{l|}{\textbf{Fine-tune}} & \multicolumn{1}{c|}{\textbf{1}} & \mc{97.5} & \mc{94.3} & \mcl{93.5} & \mc{92.2} & \mc{96.9} & \mcl{89.9} & \mc{90.4} & \mcl{90.6} & \mcl{28.0} & \mc{47.6} & \mcl{26.5} & \mctwol{\textbf{1}} & \mc{91.1} & \mc{89.7} & \mcl{87.5} & \mc{84.3} & \mc{92.0} & \mcl{70.1} & \mc{85.5} & \mc{89.9} \\ 
\midrule
% \multicolumn{1}{l|}{\textbf{Prompt}} & \multicolumn{1}{c|}{\multirow{3}{*}{\textbf{0.01}}} & \mctwo{} & \mctwo{} & \mctwo{} & \mctwo{} & \mctwol{} & \mctwo{} & \mctwol{} & \mctwol{} & \mctwo{} & \mctwo{} & \mctwol{} & \mctwo{} & \mctwo{} \\ 
\multicolumn{1}{l|}{\textbf{\AFPADJACENTExternal}} & \multicolumn{1}{c|}{\multirow{2}{*}{0.004\%}} & \mc{97.1} & \mc{92.8} & \mcl{93.6} & \mc{92.8} & \mc{96.0} & \mcl{88.8} & \mc{90.7} & \mcl{89.1} & \mcl{20.9} & \mc{49.8} & \mcl{24.0} & \mctwol{\multirow{2}{*}{0.03\%}} & \mc{87.5} & \mc{91.2} & \mcl{83.3} & \mc{82.5} & \mc{80.4} & \mcl{68.5} & \mc{84.5} & \mc{65.1} \\
\multicolumn{1}{l|}{\textbf{\AFPADJACENTInternal}} & \multicolumn{1}{c|}{} & \mc{96.2} & \mc{92.8} & \mcl{93.4} & \mc{91.4} & \mc{95.2} & \mcl{88.1} & \mc{93.7} & \mcl{87.7} & \mcl{20.9} & \mc{48.4} & \mcl{24.0} & \mctwol{} & \mc{87.1} & \mc{91.1} & \mcl{81.1} & \mc{82.0} & \mc{81.3} & \mcl{68.0} & \mc{85.8} & \mc{65.1} \\
\midrule
% \multicolumn{1}{l|}{\textbf{Bitfit}} & \multicolumn{1}{c|}{\multirow{3}{*}{\textbf{0.01}}} & \mctwo{} & \mctwo{} & \mctwo{} & \mctwo{} & \mctwol{} & \mctwo{} & \mctwol{} & \mctwol{} & \mctwo{} & \mctwo{} & \mctwol{} & \mctwo{} & \mctwo{}\\ 
\multicolumn{1}{l|}{\textbf{\AFPADJACENTExternal}} & \multicolumn{1}{c|}{\multirow{2}{*}{0.02\%}} & \mc{97.1} & \mc{89.4} & \mcl{92.9} & \mc{88.6} & \mc{96.3} & \mcl{90.7} & \mc{82.5} & \mcl{88.9} & \mcl{26.2} & \mc{50.2} & \mcl{24.8} & \mctwol{\multirow{2}{*}{0.05\%}} & \mc{89.4} & \mc{92.9} & \mcl{85.3} & \mc{84.3} & \mc{82.1} & \mcl{65.7} & \mc{86.5} & \mc{66.0} \\
\multicolumn{1}{l|}{\textbf{\AFPADJACENTInternal}} & \multicolumn{1}{c|}{} & \mc{97.3} & \mc{92.8} & \mcl{94.4} & \mc{91.4} & \mc{95.3} & \mcl{92.1} & \mc{84.6} & \mcl{87.7} & \mcl{21.4} & \mc{48.4} & \mcl{23.5} & \mctwol{} & \mc{89.4} & \mc{92.9} & \mcl{85.3} & \mc{84.3} & \mc{82.1} & \mcl{65.4} & \mc{86.0} & \mc{66.0} \\
\midrule

% \multicolumn{1}{l|}{\textbf{Lora}}
\multicolumn{1}{l|}{\textbf{\AFPADJACENTExternal}} & \multicolumn{1}{c|}{\multirow{2}{*}{0.06\%}} & \mc{97.3} & \mc{95.3} & \mcl{93.5} & \mc{91.9} & \mc{96.1} & \mcl{92.4} & \mc{92.8} & \mcl{90.6} & \mcl{23.8} & \mc{52.3} & \mcl{27.4} & \mctwol{\multirow{2}{*}{0.23\%}} & \mc{93.8} & \mc{90.0} & \mcl{88.3} & \mc{83.8} & \mc{92.3} & \mcl{74.4} & \mc{87.3} & \mc{88.9} \\
\multicolumn{1}{l|}{\textbf{\AFPADJACENTInternal}} & \multicolumn{1}{c|}{} & \mc{97.3} & \mc{92.8} & \mcl{94.4} & \mc{91.4} & \mc{95.3} & \mcl{92.1} & \mc{90.8} & \mcl{87.7} & \mcl{21.4} & \mc{48.4} & \mcl{23.5} & \mctwol{} & \mc{94.4} & \mc{89.4} & \mcl{88.7} & \mc{81.4} & \mc{90.4} & \mcl{74.7} & \mc{86.0} & \mc{85.8} \\
\midrule

% \multicolumn{1}{l|}{\textbf{Adapter}} & \multicolumn{1}{c|}{\multirow{3}{*}{\textbf{0.01}}} & \mctwo{} & \mctwo{} & \mctwo{} & \mctwo{} & \mctwol{} & \mctwo{} & \mctwol{} & \mctwol{} & \mctwo{} & \mctwo{} & \mctwol{} & \mctwo{} & \mctwo{}\\ 
\multicolumn{1}{l|}{\textbf{\AFPADJACENTExternal}} & \multicolumn{1}{c|}{\multirow{2}{*}{0.17\%}} & \mc{97.4} & \mc{93.0} & \mcl{94.1} & \mc{92.9} & \mc{96.0} & \mcl{84.5} & \mc{86.4} & \mcl{89.5} & \mcl{29.5} & \mc{49.1} & \mcl{24.3} & \mctwol{\multirow{2}{*}{0.72\%}} & \mc{92.5} & \mc{95.3} & \mcl{86.6} & \mc{87.2} & \mc{88.9} & \mcl{68.6} & \mc{86.7} & \mc{68.8} \\
\multicolumn{1}{l|}{\textbf{\AFPADJACENTInternal}} & \multicolumn{1}{c|}{} & \mc{96.3} & \mc{92.7} & \mcl{93.5} & \mc{91.1} & \mc{95.2} & \mcl{74.7} & \mc{85.6} & \mcl{88.5} & \mcl{22.8} & \mc{49.4} & \mcl{24.1} & \mctwol{} & \mc{92.5} & \mc{95.3} & \mcl{86.6} & \mc{87.2} & \mc{88.9} & \mcl{68.7} & \mc{86.6} & \mc{68.8} \\
\midrule

% \multicolumn{1}{l|}{\textbf{Prefix}} & \multicolumn{1}{c|}{\multirow{3}{*}{\textbf{0.01}}} & \mctwo{} & \mctwo{} & \mctwo{} & \mctwo{} & \mctwol{} & \mctwo{} & \mctwol{} & \mctwol{} & \mctwo{} & \mctwo{} & \mctwol{} & \mctwo{} & \mctwo{}\\ 
% \multicolumn{1}{l|}{\textbf{\AFPADJACENTExternal}} & \multicolumn{1}{c|}{\multirow{2}{*}{1.86e-02}} & \mc{97.4} & \mc{93.0} & \mcl{94.1} & \mc{92.9} & \mc{96.0} & \mcl{90.6} & \mc{86.4} & \mcl{89.5} & \mcl{30.8} & \mc{49.4} & \mcl{24.4} & \mctwol{\multirow{2}{*}{8.40e-02}} & \mc{90.5} & \mc{89.4} & \mcl{87.5} & \mc{85.0} & \mc{90.2} & \mcl{73.8} & \mc{85.5} & \mc{88.5} \\
% \multicolumn{1}{l|}{\textbf{\AFPADJACENTInternal}} & \multicolumn{1}{c|}{} & \mc{95.3} & \mc{93.7} & \mcl{93.5} & \mc{91.9} & \mc{95.9} & \mcl{88.9} & \mc{86.6} & \mcl{88.9} & \mcl{26.9} & \mc{49.8} & \mcl{24.0} & \mctwol{} & \mc{91.1} & \mc{90.0} & \mcl{86.8} & \mc{84.4} & \mc{90.5} & \mcl{74.7} & \mc{85.8} & \mc{89.5} \\
% \midrule
\bottomrule
\end{tabular}
}
\end{adjustbox}
\caption{The performance of all \AFP methods on the all investigated tasks.}
\label{appendix:table_main_results}
}
\end{table*}
